# Supplementary material for: Semiclassical Limit of Resonance States in Chaotic Scattering
Source: arXiv:2408.17088 ancillary file (2025-01-17)
Supplement: Supplementary file 1 [file Supplemental.pdf]

# Supplemental Material
# Semiclassical Limit of Resonance States in Chaotic Scattering

Roland Ketzmerick,[1] Florian Lorenz,[1] and Jan Robert Schmidt[1]

[1] *TU Dresden, Institute of Theoretical Physics and Center for Dynamics, 01062 Dresden, Germany*

(Dated: January 7, 2025)

## CONTENTS

I. Example systems and further illustrations 1
A. Dielectric cavity 2
B. Three-disk scattering system 4
C. Standard map with partial escape 6
D. Standard map with full escape 8
E. Convergence of individual resonance states 9

II. Locally randomized system and local random vector model 11
A. Locally randomized system 11
B. Local random vector model 11
1. Properties of complex random vector 11
2. Definition of transition matrix elements from local random vector 12
3. Probability distribution of transition matrix elements 13
4. Semiclassical limit 13

III. Set of nonlinear equations 14

IV. Numerical approach for determining measures 16
A. Natural decay rate 16
1. Transition time constant 16
2. Transition time not constant 16
B. Inverse natural decay rate 17
C. Arbitrary decay rate 17
1. Iterative algorithm for $\gamma \in (\gamma_{\text{nat}}, \gamma_{\text{inv}})$ 17
2. Iterative algorithm for $\gamma < \gamma_{\text{nat}}$ 18
D. Measure in position space 18

V. References 20

## I. EXAMPLE SYSTEMS AND FURTHER ILLUSTRATIONS

In the following we introduce the four example systems of the main text with all specifications needed for reproducing the classical and quantum mechanical results. Additionally, we show the spectrum of resonance poles for each system and how it relates to the chosen decay rates used in the main text. We also give visual support for the quantum-classical agreement in phase space and real space, supplementing the quantitative analysis of the main text. This includes figures for individual resonance states.

We provide Python code (as separate files) to compute $P^{\mathcal{L}}$, $P$, and $\mu$ with the methods presented in Sec. IV for all four example systems. In all examples the elements of $P^{\mathcal{L}}$ are determined using $10^4$ trajectories per cell of the partition (started on a uniform grid) for up to $n = 3200^2 \approx 10^7$ cells.

## A. Dielectric cavity

A dielectric cavity is a composition of non-magnetic, dielectric materials. Its geometry is determined by the spatial profile of the refractive index $n_{\mathrm{r}}(\boldsymbol{r})$ [1]. We here focus, as in Ref. [2], on the limaçon-shaped dielectic cavity with a constant refractive index inside ($n_{\mathrm{r}} = 3.3$ corresponding to semiconductor lasing cavities) and surrounded by vacuum ($n_{\mathrm{r}} = 1$). The boundary curve that separates both media is given in polar coordinates by $\rho(\varphi) = R_{\mathrm{cav}}(1 + \varepsilon \cos\varphi)$ with average radius $R_{\mathrm{cav}}$ and deformation parameter $\varepsilon$. For a deformation $\varepsilon = 0.6$ this is a non-convex shape and its corresponding classical billiard shows chaotic ray dynamics practically everywhere in phase space.

Energy conservation and a Poincaré surface of section at the cavity boundary allow a dimensionality reduction of the four-dimensional phase space. The resulting two-dimensional phase space is parameterized by the Birkhoff coordinates $(s, p)$. The coordinate $s \in [0, \mathcal{L}]$ gives the position along the boundary curve of length $\mathcal{L}$. The conjugate momentum $p \in [-1, 1]$ is the tangential component of the normalized momentum at a given boundary point. In this boundary phase space the time-continuous dynamics is described by a corresponding time-discrete system that maps a ray from the boundary with coordinates $(s_n, p_n)$ to its next collision $(s_{n+1}, p_{n+1})$.

When a ray hits the cavity boundary with an absolute momentum smaller than the critical value $p_{\mathrm{crit}} = n_{\mathrm{r}}^{-1}$ it divides into a reflected ray and a transmitted ray. This critical momentum value is related to the angle of total internal reflection. The momenta of the reflected and the transmitted ray are determined by the law of reflection and Snell's law, respectively. If we assign an intensity value to each ray, the intensity is then split up between the reflected ray and the transmitted ray which contributes to the farfield. The exact distribution of intensity is determined by Fresnel's law. Focusing on the inside of the cavity, we say that a ray that gets reflected and looses intensity is subject to partial escape. This is modeled by a reflection function $R^{\mathrm{TM/TE}}(p)$ defined on phase space which depends on the electromagnetic mode type one aims to describe (TM or TE). In this work we restrict ourselves to TM modes. For a more detailed description of the ray-dynamics in systems with partial escape see Ref. [1].

The limaçon billiard has a mirror-reflection symmetry with respect to the $x$-axis which can be exploited to truncate the boundary phase space to the interval $(s, p) \in \left[0, \frac{\mathcal{L}}{2}\right] \times [-1, 1]$ by applying the map

$$(s, p) \mapsto \begin{cases} (s, p)\,, & s \in \left[0, \frac{\mathcal{L}}{2}\right] \\ (\mathcal{L} - s, -p)\,, & s \in \left(\frac{\mathcal{L}}{2}, \mathcal{L}\right] \end{cases} . \tag{1}$$

This is internally used for computing $P^{\mathcal{L}}$, $P$, and $\mu$ on this desymmetrized boundary phase space. To compute the transition matrix elements $P^{\mathcal{L}}_{ji}$ we start trajectories in the Ulam cell $A_i$ (defined in the main text) and iterate them until the next boundary collision. The fraction of trajectories that end in cell $A_j$ determines $P^{\mathcal{L}}_{ji}$. The elements of the reflectivity matrix $R_{ji}$ and the transition time matrix $t_{ji}$ are given as average values over reflectivities (between 0 and 1) and transition times, respectively, again using the trajectories that start in $A_i$ and are iterated to $A_j$.

The computation of the resonance states (in this context often called modes) is based on the boundary integral approach [2]. To compare the wave solutions to our classical (ray) measure $\mu$ we average over 500 resonance modes with a similar decay rate. The modes are chosen such that the mean of their consecutive decay rates is closest to the decay rate of the classical measure. For investigating the semiclassical limit, we sequentially choose resonance modes from the intervals $\mathrm{Re}\, kR_{\mathrm{cav}} \in [100, 150]$, $[200, 250]$, $[500, 550]$, $[1000, 1050]$, $[2000, 2025]$, $[5000, 5025]$ for averaging. In Fig. S1 we show the cavity spectrum for the last interval $\mathrm{Re}\, kR_{\mathrm{cav}} \in [5000, 5025]$. The imaginary part of the wave number $k$ is related to the decay rate $\gamma$ by $\mathrm{Im}\, kR_{\mathrm{cav}} = -\frac{\gamma\tau}{2}$, where we set the time scale $\tau = 1$. Poles used for averaging are highlighted.

For several decay rates a comparison between the averaged resonance modes and the classical measure $\mu$ is shown in Fig. S2 for (a) the Husimi representation on the boundary phase space and (b) in position space. The measure in phase space is smoothed on the scale of the wavelength. The Husimi representation is evaluated on a $3200 \times 3200$ grid on the full boundary phase space for various $kR_{\mathrm{cav}}$. The observed agreement is perfect and visualizes the quantitative correspondence from the main text.

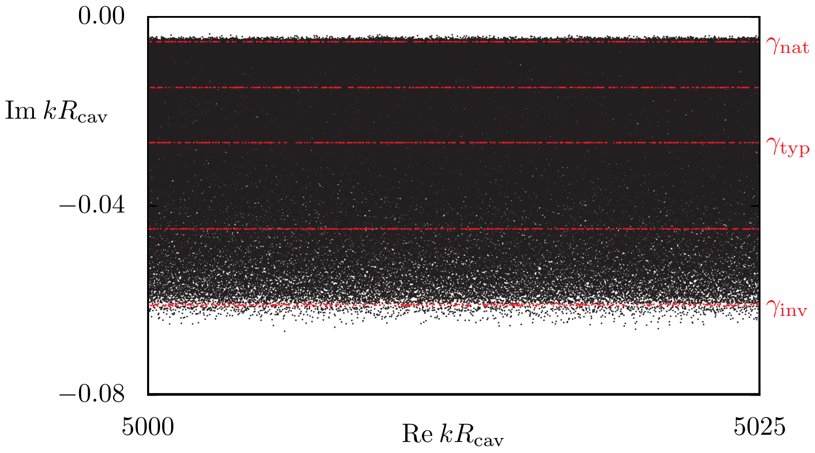


FIG. S1. Spectrum of the dielectric cavity for antisymmetric TM-modes with $\varepsilon = 0.6$ at $\mathrm{Re}\, kR_{\mathrm{cav}} \in [5000, 5025]$ and $\mathrm{Im}\, kR_{\mathrm{cav}} \in [-0.08, 0]$, showing about 400000 poles. The poles corresponding to resonance states used for averaging in Fig. S2 are marked in red.

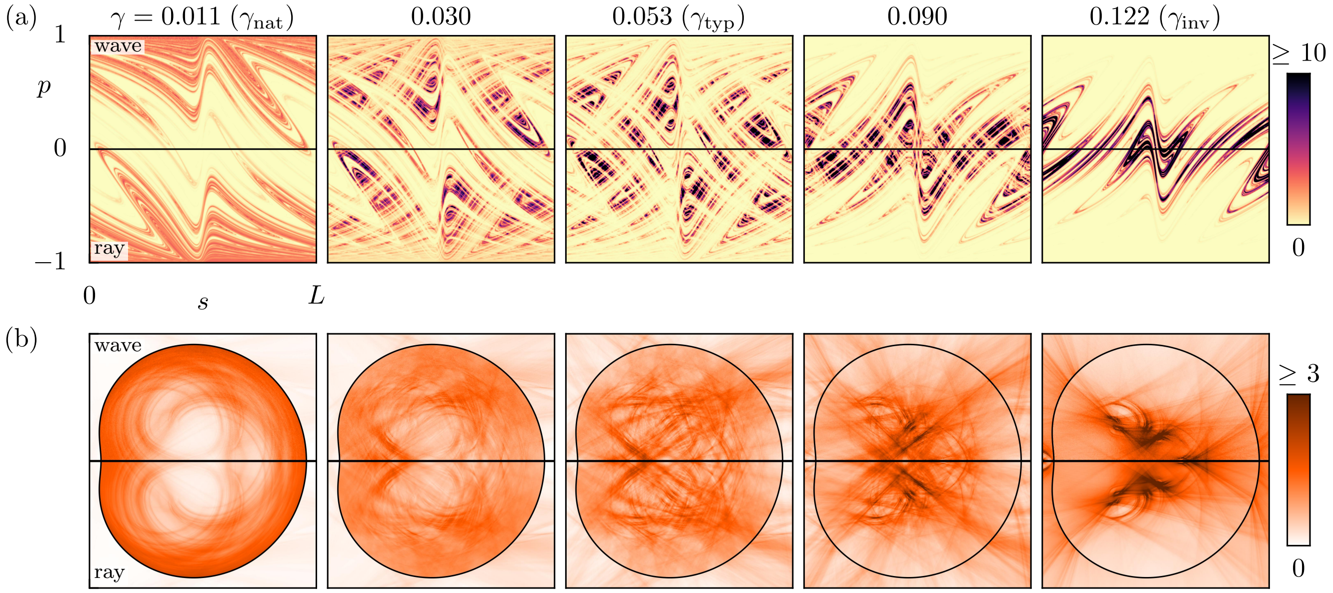


FIG. S2. Conditionally invariant measure $\mu$ for finest partition ($n = 3200^2 \approx 10^7$) proposed in main text (ray) compared to averaged resonances states (wave) in (a) Husimi representation on boundary phase space and (b) position space. Averages are taken over 500 resonance states with imaginary part close to five representative values of $\mathrm{Im}\, kR_{\mathrm{cav}}$, where $\mathrm{Re}\, kR_{\mathrm{cav}} \in [5000, 5025]$ and $\gamma \in \{0.011, 0.03, 0.053, 0.09, 0.012\}$. In all figures the average value (in (a) on the boundary phase space, in (b) on the inside of the cavity) is scaled to one and intensities greater than the maximal value of the color bar are shown with darkest color.

### B. Three-disk scattering system

The three-disk scattering system is an autonomous system with two degrees of freedom and full escape. It consists of three hard disks of radius $a$ with centers at the corners of an equilateral triangle of side length $R_{\mathrm{3disk}}$. Here we use the dimensionless ratio $R_{\mathrm{3disk}}/a = 2.1$ which uniquely characterizes the system. A point particle moves along straight lines between collisions with the disks and is specularly reflected at their boundaries. The dynamics is chaotic with no stable periodic orbits present. Using the systems $C_{3\mathrm{v}}$ symmetry, the dynamics can be reduced to a fundamental domain. For background on the three-disk scattering system, the parameter choice, and the structure of its resonance states see Ref. [3].

The phase space is reduced by a Poincaré surface of section at one disk's boundary and parametrized by dimensionless Birkhoff coordinates $(s, p)$. We confine our analysis to the region $s \in \left[-\frac{2}{3}\pi, \frac{2}{3}\pi\right]$ and $p \in [-1, 1]$, which ensures that all trajectories with at least two reflections are included. Using symmetry, we further reduce the boundary phase space to the region $s \in \left[0, \frac{2}{3}\pi\right]$ and $p \in [-1, 1]$ for computing $P^{\mathcal{L}}$, $P$, and $\mu$. This corresponds to the fundamental domain of the system and reduces the computational cost by a factor of 2.

In addition to the cells of the partition of the boundary phase space one further cell at infinity would be needed for trajectories leaving the system. However, to simplify the computation, we count for the transition matrix $P^{\mathcal{L}}$ such trajectories as going to the cell with inverted direction of momentum, i.e. as if they were reflected at infinity. This cell has zero measure anyway. The reflectivity matrix element $R_{ji}$ is set to 0 in this case, otherwise it is 1. The transition times $t_{ji}$ are determined by averaging over the points mapped from cell $A_i$ to $A_j$. The final measure $\mu$ is multiplied by $\sqrt{1-p^2}$ to follow the properties of the usual definition of the boundary Husimi representation.

The resonances poles, resonances states, and their representation in the position space and Husimi representation on the boundary phase space are computed in the $\mathrm{A}_2$ symmetry class using a method introduced in Ref. [3] with Python code provided therein. For comparison to the measure $\mu$ introduced in the main text, we use intervals of resonances at $\mathrm{Re}\, ka \in [1000, 5000]$, $[5000, 8000]$, $[10000, 12000]$, $[20000, 21000]$, $[50000, 50500]$, $[100000, 100200]$. The spectrum in the interval at largest $\mathrm{Re}\, ka$ is shown in Fig. S3. The imaginary part of the wave number $k$ is related to the decay rate $\gamma$ by $\mathrm{Im}\, ka = -\frac{\gamma\tau}{2}$, where we set the time scale $\tau = 1$. To illustrate the agreement of the measure $\mu$ with the resonance states, we average over the 500 consecutive states with average decay rate closest to the desired decay rate. For the interval $\mathrm{Re}\, ka \in [100000, 100200]$ these poles are highlighted in Fig. S3. In this interval with highest $\mathrm{Re}\, ka$ the fast decaying poles around $\mathrm{Im}\, ka = -0.9$ (corresponding to $\gamma = 1.8$) could not be computed with sufficient precision. The corresponding resonance states are thus not included in the comparison of Fig. 4(b) of the main text.

In Fig. S4 we compare the average over 500 resonance states in (a) Husimi representation on the boundary phase space and (b) position space with the measure $\mu$ for several decay rates. The measure is smoothed on the scale of the Planck cell of the corresponding resonance states. We compute the Husimi function on a grid of $6400 \times 3200$ points for $s \in \left[-\frac{2}{3}\pi, \frac{2}{3}\pi\right]$ and $p \in [-1, 1]$. The observed agreement is perfect and visualizes the quantitative correspondence from the main text.

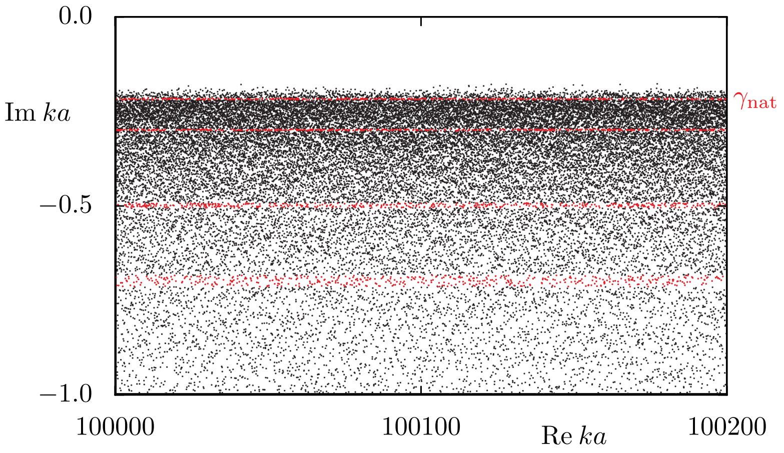


FIG. S3. Spectrum of the three-disk scattering system with $R_{\rm 3disk}/a = 2.1$ at $\mathrm{Re}\, ka \in [100000, 100200]$ and $\mathrm{Im}\, ka \in [-1, 0]$, showing about 35000 poles. The poles corresponding to resonance states used for averaging in Fig. S4 are marked in red.

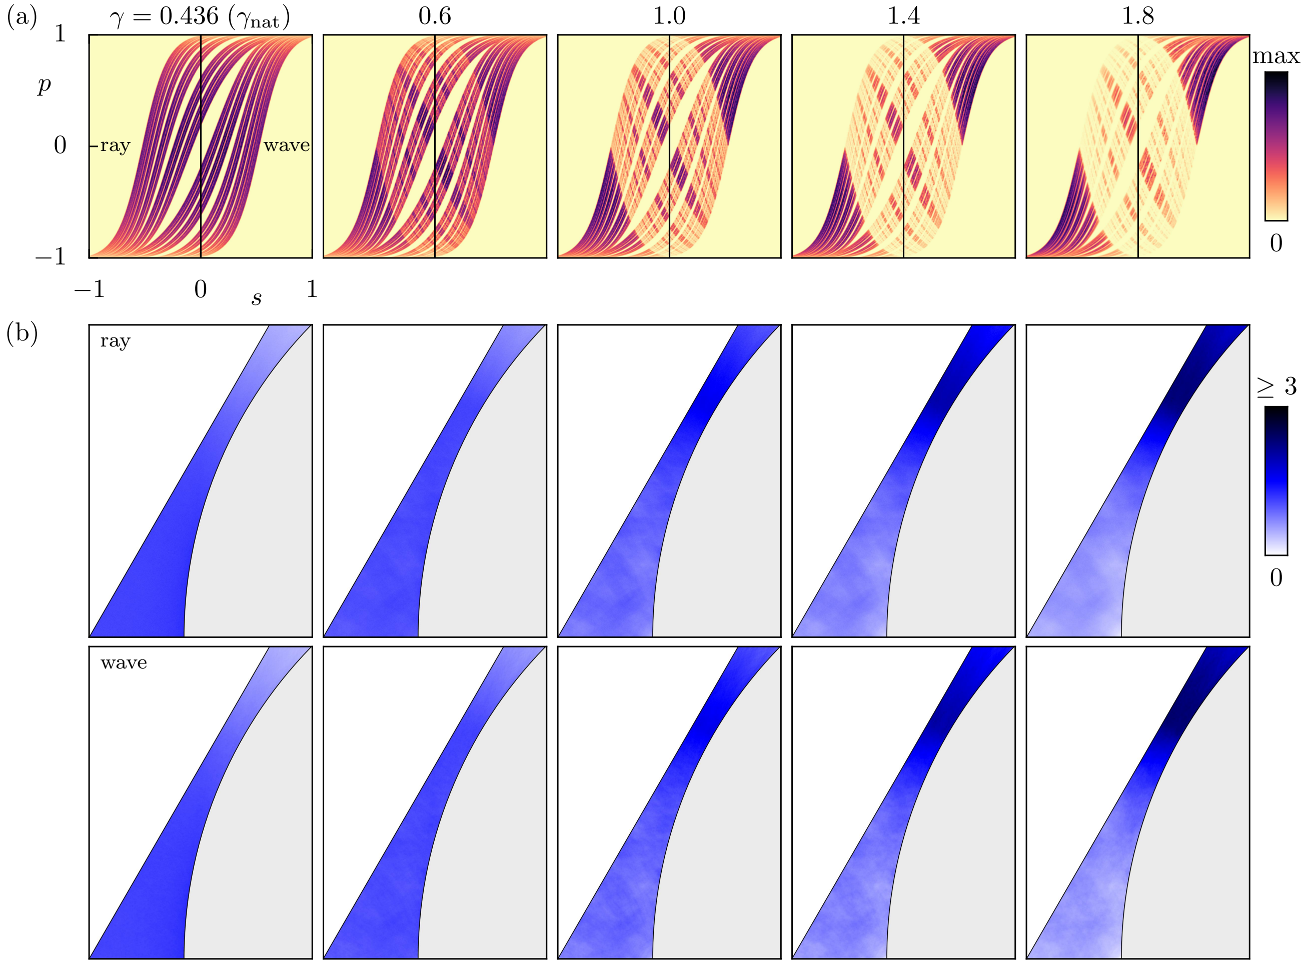


FIG. S4. Conditionally invariant measure $\mu$ for finest partition ($n = 3200^2 \approx 10^7$) proposed in main text (ray) compared to averaged resonances states (wave) in (a) Husimi representation on boundary phase space and (b) position space in fundamental domain confined to a region of size $0.5a \times 0.7a$. Averages are taken over 500 resonance states with imaginary part close to five representative values of $\mathrm{Im}\, ka$. Specifically, in (a) $\mathrm{Re}\, ka \in [100000, 100200]$ for $\gamma \in \{0.436, 0.6, 1.0, 1.4\}$ and $\mathrm{Re}\, ka \in [50000, 50500]$ for $\gamma = 1.8$ and in (b) $\mathrm{Re}\, ka \in [20000, 21000]$ for all $\gamma$. In all figures the average value is scaled to one, in (a) on backward-trapped set, in (b) on shown region of fundamental domain. In (a) the maxima are approximately given by 2.4, 2.9, 4.2, 5.5, and 6.8 (from left to right). In (b) intensities greater than the maximal value of the color bar are shown with darkest color.

### C. Standard map with partial escape

The standard map is a two-dimensional symplectic map showing a variety of dynamics ranging from integrable to fully chaotic [4]. Here we consider its symmetrized version at half-kick,

$$q_{n+1} = q_n + p^* \tag{2}$$
$$p_{n+1} = p^* - V'(q_{n+1})/2, \tag{3}$$

where $p^* = p_n - V'(q_n)/2$, the potential is $V(q) = K/(4\pi^2)\cos(2\pi q)$ with kicking strength $K$, and phase space coordinates $(q,p) \in [0,1) \times [0,1)$ with periodic boundary conditions. In this paper we use $K = 10$, where the dynamics is practically fully chaotic. This allows for computing the Lebesgue transition matrix $P^{\mathcal{L}}$.

For considering partial escape, we introduce a region $\Omega$ in phase space where the reflectivity is reduced to $R_\Omega = 0.2$, such that

$$R(q) = \begin{cases} R_\Omega & \text{for } q \in [0.3, 0.6) \\ 1 & \text{otherwise.} \end{cases} \tag{4}$$

The reflectivity matrix elements $R_{ji}$ are determined by averaging over the reflectivity function $R(q)$ evaluated for the points mapped from cell $A_i$ to $A_j$.

The quantum time evolution of the closed standard map is given by [5, 6]

$$\mathcal{U}_{\text{cl}} = \mathrm{e}^{-\mathrm{i}/(2\hbar)V(\hat{q})}\mathrm{e}^{-\mathrm{i}/(2\hbar)\hat{p}^2}\mathrm{e}^{-\mathrm{i}/(2\hbar)V(\hat{q})}, \tag{5}$$

where $h = 2\pi\hbar$ is the effective Planck constant, such that $h \to 0$ is the semiclassical limit. As we use periodic boundary conditions, only discrete values $h = 1/N$ with $N \in \mathbb{N}$ are allowed. Escape is introduced through the projective coupling operator

$$\mathcal{R} = \mathcal{P}_{\Omega^c} + \sqrt{R_\Omega}\mathcal{P}_\Omega, \tag{6}$$

resulting in the subunitary time evolution operator $\mathcal{U} = \mathcal{U}_{\text{cl}}\,\mathcal{R}$. Therefore, the eigenvalues $\lambda = \mathrm{e}^{\mathrm{i}\theta - \gamma/2}$ of $\mathcal{U}$ have modulus less than one, i.e. decay rates $\gamma > 0$.

For comparison to the measure $\mu$ introduced in the main text, we average over poles from matrices, whose sizes $N$ correspond to all even numbers in the intervals $N \in [400, 600]$, $[940, 1060]$, $[1960, 2040]$, $[4980, 5020]$, $[9990, 10010]$, $[19996, 20004]$. The spectrum from the interval $N \in [19996, 20004]$ is shown in Fig. S5. To illustrate the agreement of the measure $\mu$ with the resonance states, we average over the 500 consecutive states with average decay rate closest to the desired decay rate. For the interval $N \in [19996, 20004]$ these poles are highlighted in Fig. S5.

In Fig. S6 we compare the average over 500 resonance states in Husimi representation on the phase space with the measure $\mu$ for several decay rates. The measure is smoothed on the scale of the Planck cell of the corresponding resonance states. We compute the Husimi function on a grid of $3200 \times 3200$ points for all $N$. The observed agreement is perfect and visualizes the quantitative correspondence from the main text.

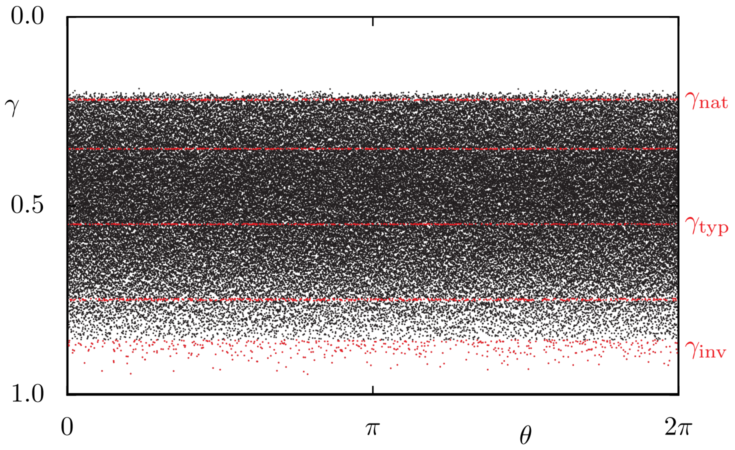


FIG. S5. Spectrum of the standard map with partial escape for all even $N \in [19996, 20004]$ and parameters given in the text. The poles corresponding to resonance states used for averaging in Fig. S6 are marked in red.

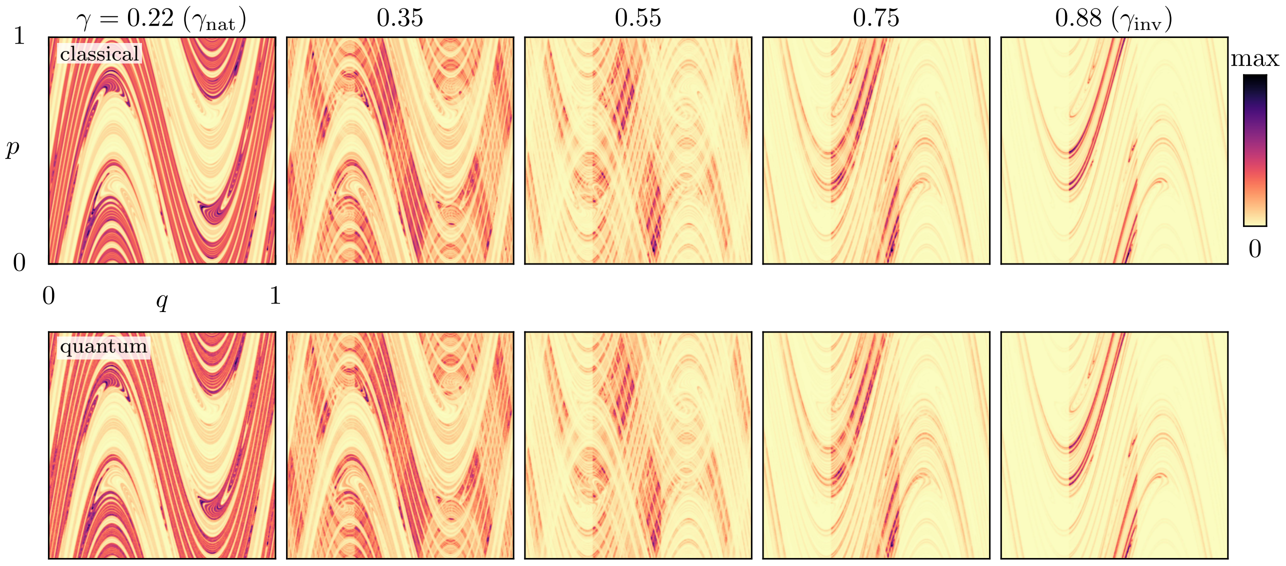


FIG. S6. Conditionally invariant measure $\mu$ for finest partition ($n = 3200^2 \approx 10^7$) proposed in main text (classical, top) compared to averaged resonances states (quantum, bottom) in Husimi representation. Averages are taken over 500 resonance states with decay rates close to five representative values of $\gamma$, for all even $N \in [19996, 20004]$. In all figures the average value is scaled to one. The maxima are approximately given by 5.5, 7.9, 15.8, 23.5, and 39.2 (from left to right).

### D. Standard map with full escape

We also consider the standard map with full escape, i.e., the map as introduced in the previous section I C with $R_\Omega = 0$. The spectrum from the interval $N \in [19996, 20004]$ is shown in Fig. S7. To illustrate the agreement of the measure $\mu$ with the resonance states, we average over the 500 consecutive states with average decay rate closest to the desired decay rate. For the interval $N \in [19996, 20004]$ these poles are highlighted in Fig. S7.

In Fig. S8 we compare the average over 500 resonance states in Husimi representation on the phase space with the measure $\mu$ for several decay rates. The observed agreement is perfect and visualizes the quantitative correspondence from the main text.

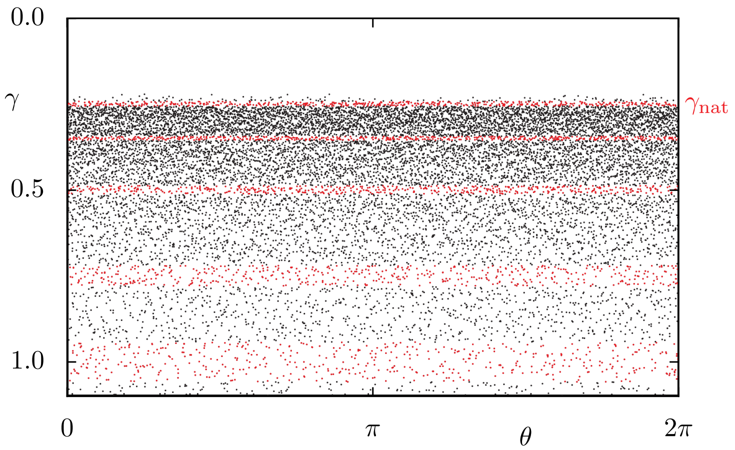


FIG. S7. Spectrum of the standard map with full escape for all even $N \in [19996, 20004]$ and parameters given in the text. The poles corresponding to resonance states used for averaging in Fig. S8 are marked in red.

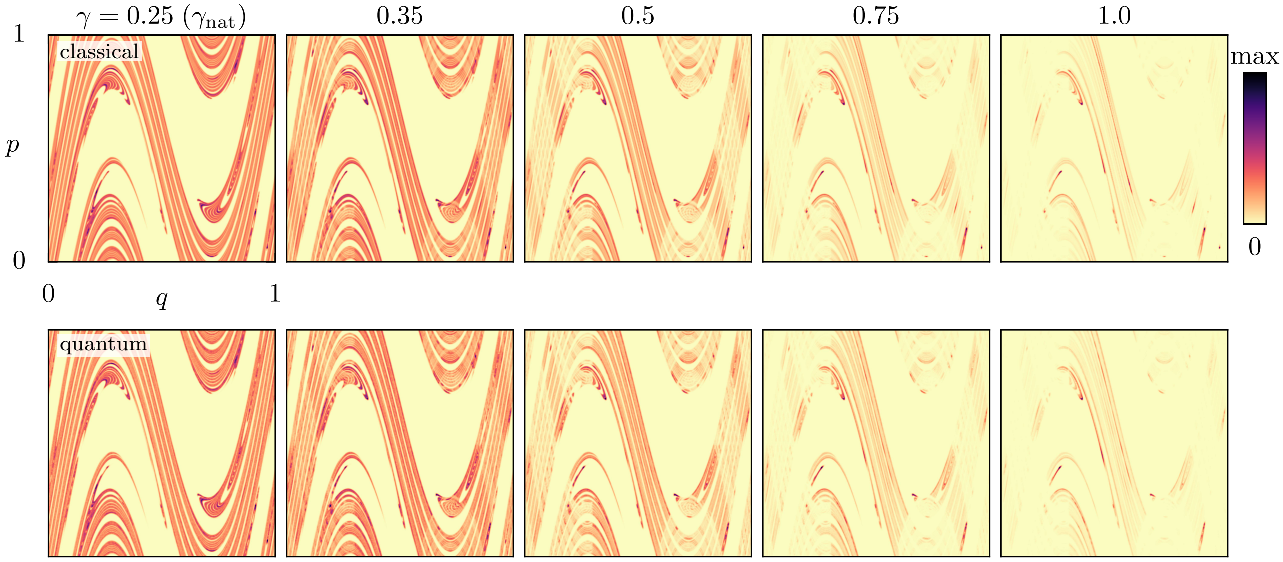


FIG. S8. Same as Fig. S6 but for the standard map with full escape. In all figures the average value is scaled to one on the backward-trapped set. The maxima are approximately given by 5.9, 6.9, 13.1, 32.1, and 70.3 (from left to right).

### E. Convergence of individual resonance states

In Fig. 4 of the main text we show the convergence of averaged resonance states to the proposed conditionally invariant measure $\mu$. Here we illustrate the convergence of individual resonance states to $\mu$ in the semiclassical limit. To this end we compute the Jensen-Shannon divergence $d_{\mathrm{JS}}$ between the Husimi representation of the individual resonance states and the measure $\mu$ for several wavelengths and all systems as in the main text, see Fig. S9. This shows that individual resonance states also converge to $\mu$ in the semiclassical limit. However, the Jensen-Shannon divergence is much larger than in Fig. 4 of the main text for averaged resonance states. This is due to the fluctuations of individual resonance states.

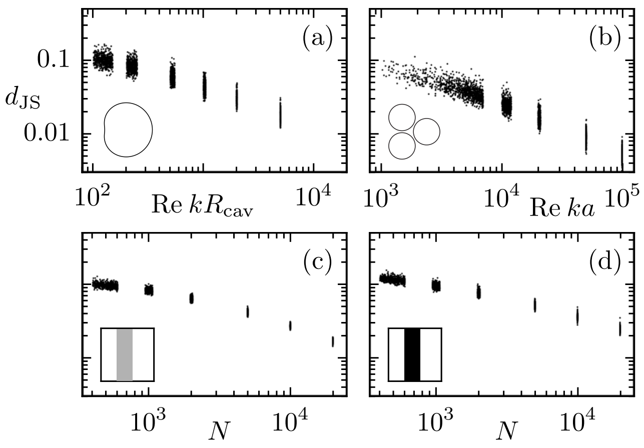


FIG. S9. Convergence of individual resonance states to conditionally invariant measures with $n = 3200^2 \approx 10^7$ for systems and third decay rate of Fig. 4 in the main text. Shown is the decay of the Jensen-Shannon divergence $d_{\mathrm{JS}}$ in the semiclassical limit, i.e. (a, b) increasing wave number $\mathrm{Re}\, k$ or (c, d) matrix size $N$.

Furthermore, we illustrate individual resonance state and compare them to the proposed conditionally invariant measure $\mu$, see for each example system in Figs. S10, S11, S12, and S13. These figures each correspond to one data point at small wavelength in Fig. S9(a-d). Due to the fluctuations of an individual resonance state this comparison is a much less sensitive test for the quality of the selected measure.

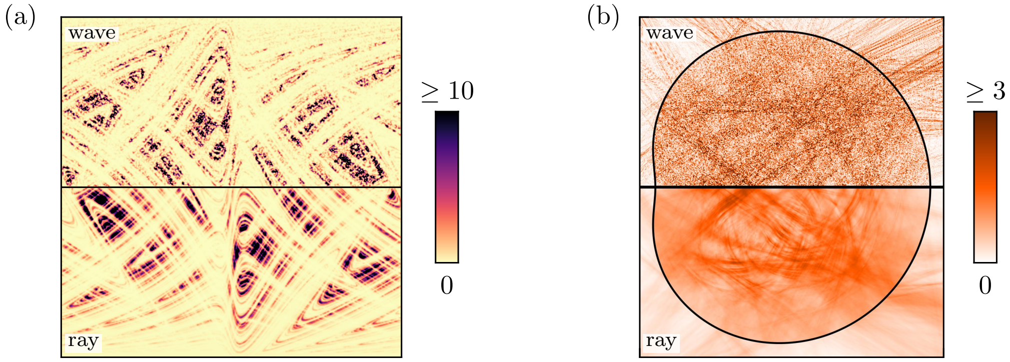


FIG. S10. Dielectric cavity: Conditionally invariant measure $\mu$ proposed in main text (bottom, ray) compared to one individual resonances state near $\gamma = 0.053$ (top, wave) in (a) Husimi representation on boundary phase space and (b) position space on a $500 \times 560$ grid with grid distance of 11.7 wavelengths. The resonance state is taken from the interval $\mathrm{Re}\, ka \in [5000, 5025]$. This visualizes the comparison for one of the data points in Fig. S9(a). Further details as in Fig. S2.

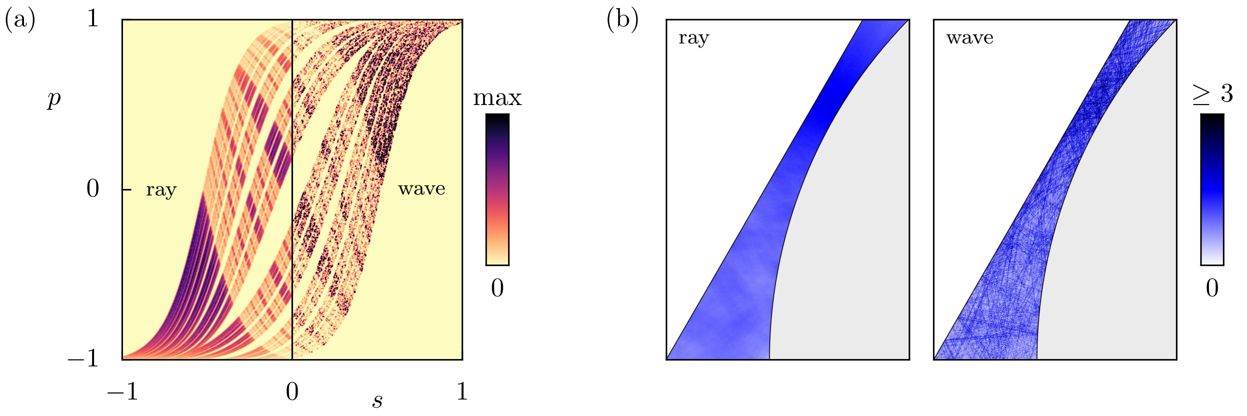


FIG. S11. Three-disk scattering system: Conditionally invariant measure $\mu$ proposed in main text (left, ray) compared to one individual resonances state (right, wave) near $\gamma = 1.0$ in (a) Husimi representation on boundary phase space and (b) position space on a $500 \times 700$ grid with grid distance of 3.3 wavelengths. The resonance state is taken from the interval (a) $\mathrm{Re}\, ka \in [100000, 100200]$ and (b) $\mathrm{Re}\, ka \in [20000, 21000]$. This visualizes the comparison for one of the data points in Fig. S9(b). Further details as in Fig. S4.

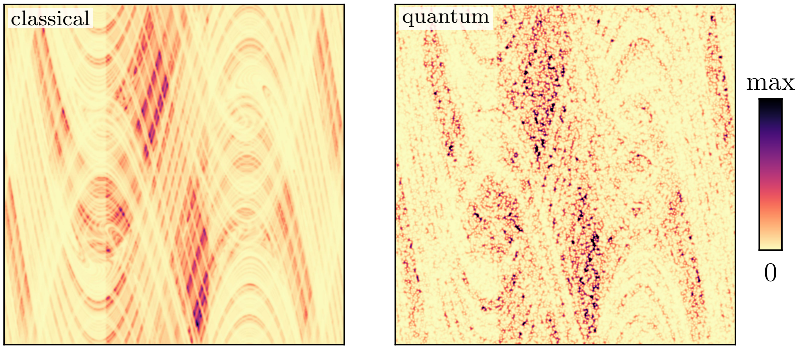


FIG. S12. Standard map with partial escape: Conditionally invariant measure $\mu$ proposed in main text (classical, left) compared to individual resonances state (quantum, right) in Husimi representation near $\gamma = 0.55$. The resonance state is taken from the interval $N \in [19996, 20004]$. This visualizes the comparison for one of the data points in Fig. S9(c). Further details as in Fig. S6.

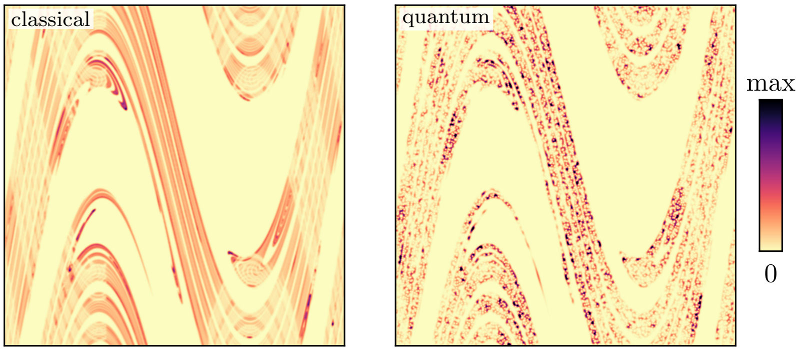


FIG. S13. Standard map with full escape: Same as Fig. S12 but for full escape near $\gamma = 0.5$. This visualizes the comparison for one of the data points in Fig. S9(d). Further details as in Fig. S8.

## II. LOCALLY RANDOMIZED SYSTEM AND LOCAL RANDOM VECTOR MODEL

### A. Locally randomized system

In Ref. [7] a *locally randomized* Baker map with escape was introduced and studied. It was shown that its resonance states are perfectly described by a local random vector model. In this section these ideas of Ref. [7] are generalized to other scattering systems. This supports the remark in the main text that the selection criterion for the transition matrix (closeness to the Lebesgue transition matrix in terms of the Kullback-Leibler divergence) can be derived for locally randomized scattering systems.

A locally randomized quantum map can be generated by multiplying the time evolution operator of a quantum map with escape (in our case a subunitary matrix) with a randomization operator. The randomization is done on a grid in phase space by locally multiplying each grid region with a random matrix taken from the circular unitary ensemble [7, Sec. 3.2]. The dimension of each random matrix must be chosen such that, multiplied by the number of randomization regions, it gives the dimension of the system Hilbert space. For the following it is preferable to place the randomization operator to the left of the system operator (in Ref. [7] the other order was used). Note that the randomization is well defined and can be numerically implemented for maps, while for scattering systems like a dielectric cavity or the three-disk scattering system we use it as a conceptual idea.

The locally randomized system is an auxiliary system of no physical interest by itself. What is the motivation to study it?

(i) Its resonance states have the property that in the semiclassical limit the scale of the Planck cell is separated from the scale of classical phase-space structures. This is an advantage compared to the resonance states of the original deterministic system, where the fractal structure continues all the way to the Planck cell, independent of how far in the semiclassical limit the system is studied. In fact, the resonance states of a randomized system, with randomization regions given by the cells $A_i$ of a partition, are uniform in each subregion $A_{ji}$ (with just universal fluctuations on smaller scales). In the semiclassical limit this structure does not change for resonance states with similar decay rate. It turns out that the weights on each subregion $A_{ji}$ can be found with the help of a local random vector model, as described below in Sec. II B. The result is found to be equivalent to the conjecture in the main text about the selection criterion for the transition matrix, namely closeness to the Lebesgue transition matrix in terms of the Kullback-Leibler divergence.

(ii) One can hope that resonance states of the randomized system have the same properties as resonance states with similar decay rate of the original deterministic system, if the following limits are taken in the right order. One considers properties on a fixed classical scale and studies the semiclassical limit for increasingly smaller randomization regions. Unfortunately, this hope was not fulfilled for the randomized Baker map, where small deviations in the properties of its resonance states compared to the deterministic Baker map appeared [7]. We now attribute this to anomalies due to the discontinuity of the Baker map. Due to the success of the selection criterion in the main text, we expect that for other scattering systems than the Baker map, there is agreement between resonance states of the randomized and the deterministic system. The numerical support of these ideas needs future studies.

### B. Local random vector model

A local random vector model has been used in Ref. [7, Sec. 4.2] to describe resonance states of the randomized Baker map with escape. For general random vector models, see Refs. [8–10]. For the Baker map the partition was chosen in Ref. [7], such that any cell $A_i$ has subregions $A_{ji}$ (see main text) of the same size and same number. Here we generalize this local random vector model to an arbitrary number and size of subregions $A_{ji}$ with $\bigcup_j A_{ji} = A_i$. We use the notation of the main text.

#### 1. *Properties of complex random vector*

We define a complex random vector $(c_1, c_2, \ldots, c_N) \in \mathbb{C}^N$ of dimension $N \gg 1$. Its complex components $c_k$ are normalized,

$$\sum_{k=1}^{N} |c_k|^2 = 1 , \tag{7}$$

and otherwise independent, such that their joint probability distribution is proportional to [8–10]

$$P(c_1, c_2, \ldots, c_N) \propto \delta\left(1 - \sum_{k=1}^{N} |c_k|^2\right) , \tag{8}$$

where the prefactors depending on $N$ for normalization are ignored. We define the absolute squared value of each complex component,

$$y_k = |c_k|^2 . \tag{9}$$

They can be shown to have the joint probability distribution,

$$P(y_1, y_2, \ldots, y_N) \propto \delta\left(1 - \sum_{k=1}^{N} y_k\right) , \tag{10}$$

up to prefactors with the normalization restriction,

$$\sum_{k=1}^{N} y_k = 1 . \tag{11}$$

The straightforward derivation uses

$$\int_{-\infty}^{\infty} \mathrm{d}(\mathrm{Re}\, c_k) \int_{-\infty}^{\infty} \mathrm{d}(\mathrm{Im}\, c_k) \quad \ldots \quad = \int_{0}^{2\pi} \mathrm{d}\varphi_k \int_{0}^{\infty} \mathrm{d}z_k \; z_k \quad \ldots \quad = \pi \int_{0}^{\infty} \mathrm{d}y_k \quad \ldots , \tag{12}$$

where in the first step polar coordinates in the complex plane are used with $c_k = z_k \mathrm{e}^{\mathrm{i}\varphi_k}$. In the second step a change of variables to $y_k = z_k^2$ and the independence of the argument on $\varphi_k$ is used.

Below, we will need the joint probability distribution for partial sums $p_j = \sum_{k \in K_j} y_k$ from disjoint index sets $K_j$ each with $m_j$ elements, such that $\sum_j p_j = 1$, $\sum_j m_j = N$, and $\bigcup_j K_j = \{1, 2, \ldots, N\}$. Up to prefactors it is given by

$$P\left(p_1, p_2, \ldots\right) \propto \prod_j p_j^{m_j - 1} . \tag{13}$$

This result follows from Eq. (10), i.e. a uniform distribution on the surface of an $N$ dimensional simplex, and that each partial sum defines the surface of an $m_j$ dimensional simplex of extent $p_j$ in each dimension.

### 2. *Definition of transition matrix elements from local random vector*

The $N$ components $c_k$ of the random vector are now associated with a single cell $A_i$. This is the reason why we use the term *local* random vector model. We place the components of the vector uniformly within the cell $A_i$, i.e. in accordance with the Lebesgue transition matrix $P_{ji}^{\mathcal{L}} = \mu_{\mathcal{L}}(A_{ji}) \;/\; \mu_{\mathcal{L}}(A_i)$, defined in the main text. Therefore in subregion $A_{ji}$ there are approximately

$$N_{ji} \approx P_{ji}^{\mathcal{L}} N \tag{14}$$

components $c_k$. Their indices $k$ define a set $\mathcal{K}_{ji}$.

We define transition matrix elements $P_{ji}$ for fixed $i$ from the local random vector by the norm of the random vector within subregion $A_{ji}$,

$$P_{ji} = \sum_{k \in \mathcal{K}_{ji}} |c_k|^2 = \sum_{k \in \mathcal{K}_{ji}} y_k . \tag{15}$$

From this definition follows that $\sum_j P_{ji} = 1$, as required for a transition matrix, because $\bigcup_j \mathcal{K}_{ji}$ is the set of all indices $1, 2, \ldots, N$ and there is normalization, Eq. (7).

Using independent local random vectors for all cells $A_i$, defines all matrix elements $P_{ji}$. Note that a global random vector for the entire system would not fulfill the normalization in each cell and thus not lead to transition matrix elements fulfilling $\sum_j P_{ji} = 1$ for all $i$.

### *3. Probability distribution of transition matrix elements*

The joint probability distribution $P(\{P_{ji}; \forall j\})$ of all transition matrix elements $P_{ji}$ for a fixed cell $A_i$ is given by the probability of the corresponding local random vector to fulfill Eq. (15). According to Eq. (13) we thus have for a fixed cell $A_i$,

$$P(\{P_{ji}; \forall j\}) \propto \prod_j P_{ji}^{N_{ji}-1} \approx \prod_j P_{ji}^{P_{ji}^{\mathcal{L}} N} , \tag{16}$$

where in the last step we used $N_{ji} \gg 1$ and Eq. (14). Using independent local random vectors for all cells $A_i$, the joint probablity distribution for *all* transition matrix elements $P_{ji}$ is the product,

$$P(\{P_{ji}; \forall i, j\}) \propto \prod_{i,j} P_{ji}^{P_{ji}^{\mathcal{L}} N} = \left( \prod_{i,j} P_{ji}^{P_{ji}^{\mathcal{L}}} \right)^N . \tag{17}$$

### *4. Semiclassical limit*

In the semiclassical limit $N \to \infty$ the joint probability distribution, Eq. (17), gets increasingly peaked at the maximum of $\prod_{i,j} P_{ji}^{P_{ji}^{\mathcal{L}}}$, leading effectively to a delta function. This selects a specific transition matrix $P_{ji}$.

The location of the maximum is unchanged, if instead we maximize the logarithm of the probability distribution, giving the simpler expression to be maximized,

$$\sum_{i,j} P_{ji}^{\mathcal{L}} \ln P_{ji} . \tag{18}$$

This is equivalent to *minimizing* the Kullback-Leibler divergence, given in the main text, which has a different sign. Further differences, the prefactor and the additional constant term $\sum_{i,j} P_{ji}^{\mathcal{L}} \ln P_{ji}^{\mathcal{L}}$, are irrelevant.

Note that if every cell $A_i$ has subregions $A_{ji}$ of the same size and the same number, the Lebesgue transition matrix has just constant elements (or they are zero). In this special case of the Baker map the results of Ref. [7, Sec. 4.2] are recovered.

## III. SET OF NONLINEAR EQUATIONS

Here we describe how the selection of the transition matrix $P$ for a given decay rate $\gamma$ leads to a set of nonlinear equations. The unknown transition matrix $P$ has the property,

$$\sum_j P_{ji} = 1 \quad \forall i \; . \tag{19}$$

The coarse-grained conditionally invariant measure $\mu$ has to fulfill the following constraints, see main text,

$$\sum_i P_{ji} Z_{ji} \; \mu_i = \mu_j \quad \forall j \tag{20}$$

$$\sum_i \mu_i = 1 \; , \tag{21}$$

where we used the abbreviation

$$Z_{ji} = R_{ji} \mathrm{e}^{\gamma t_{ji}} \; , \tag{22}$$

with the given decay rate $\gamma$.

Under these three constraints, Eq. (19) to Eq. (21), we want to minimize the Kullback-Leibler divergence from $P$ to $P^{\mathcal{L}}$, see main text,

$$d(P^{\mathcal{L}}||P) = \frac{1}{n} \sum_i \left( - \sum_j P^{\mathcal{L}}_{ji} \ln \frac{P_{ji}}{P^{\mathcal{L}}_{ji}} \right) \; . \tag{23}$$

This is equivalent to finding the extremum of the following function with Lagrange multipliers $x_i$, $y_i$, and $z$,

$$\begin{aligned} f(\{P_{ji}\}, \{\mu_i\}, \{x_i\}, \{y_i\}, z) = & \sum_{i,j} P^{\mathcal{L}}_{ji} \ln P_{ji} \\ & - \sum_i x_i \left( \sum_j P_{ji} - 1 \right) \\ & - \sum_j y_j \left( \sum_i P_{ji} Z_{ji} \mu_i - \mu_j \right) \\ & - z \left( \sum_i \mu_i - 1 \right) \; . \end{aligned} \tag{24}$$

At the extremum the derivative with respect to all variables $P_{ji}$ and $\mu_i$ is zero, leading to

$$P_{ji} \left( x_i + y_j Z_{ji} \mu_i \right) = P^{\mathcal{L}}_{ji} \qquad \forall i, j \tag{25}$$

$$\sum_j y_j P_{ji} Z_{ji} = y_i - z \qquad \forall i \tag{26}$$

in addition to the constraints Eqs. (19) to (21). We now eliminate the Lagrange multipliers $z$ and $x$. First, we multiply Eq. (26) by $\mu_i$ and sum over $i$ leading to

$$\sum_j y_j \sum_i P_{ji} Z_{ji} \mu_i = \sum_i y_i \mu_i - z \sum_i \mu_i \; , \tag{27}$$

which by using Eq. (20) gives $z = 0$ and simplifies Eq. (26) to

$$\sum_j y_j \; P_{ji} Z_{ji} = y_i \qquad \forall i \; . \tag{28}$$

We see that the Lagrange multiplier $y$ is proportional to the left eigenvector of $P_{ji} Z_{ji}$. Note that this does not correspond to the left resonance state of the quantum system, unless for $\gamma = \gamma_{\mathrm{nat}}$.

Secondly, we sum Eq. (25) over $j$ and use that $P$ and $P^{\mathcal{L}}$ are transition matrices, Eq. (19), as well as Eq. (28), leading to,

$$x_i + y_i \mu_i = 1 \qquad \forall i \ , \tag{29}$$

which can be used to eliminate $x_i$ in Eq. (25),

$$P_{ji} \left(1 - y_i \mu_i + y_j Z_{ji} \mu_i\right) = P^{\mathcal{L}}_{ji} \quad \forall i, j \ . \tag{30}$$

Finally, grouping together Eq. (30) and the three constraints Eqs. (19) to (21), we have the following set of nonlinear equations,

$$P_{ji} = \frac{P^{\mathcal{L}}_{ji}}{1 + \left(y_j Z_{ji} - y_i\right) \mu_i} \qquad \forall i, j \tag{31}$$

$$\sum_j P_{ji} = 1 \qquad \forall i \tag{32}$$

$$\sum_i P_{ji} Z_{ji} \ \mu_i = \mu_j \qquad \forall j \tag{33}$$

$$\sum_i \mu_i = 1 \ , \tag{34}$$

with the unknown variables $P_{ji}$, $\mu_i$, and $y_i$. If the set of nonlinear equations has more than one solution, the one with the smallest Kullback-Leibler divergence has to be chosen.

Let us finish this section with a couple of remarks on the set of nonlinear equations:

1. At the natural decay rate, $\gamma = \gamma_{\text{nat}}$, we have $y \equiv 0$ and $P_{ji} = P^{\mathcal{L}}_{ji}$ and thus $\mu = \mu_{\text{nat}}$.

2. For systems with partial escape at the inverse decay rate, $\gamma = \gamma_{\text{inv}}$, we find that $y_i = 1/\mu_i$ fulfills the nonlinear equations with $P_{ji} = P^{\mathcal{L}}_{ji} \mu_j / (Z_{ji} \mu_i)$. In particular, Eq. (32) leads to $\sum_j (1/Z_{ji}) P^{\mathcal{L}}_{ji} \mu_j = \mu_i$, which corresponds to the backward dynamics with the inverse reflection coefficients previously used [11] to find $\mu = \mu_{\text{inv}}$.

3. In the case of full escape there are cells $j$ with $\mu_j = 0$ and thus the corresponding Lagrange multiplier $y_j$ in Eq. (24) is undefined. As a consequence, Eq. (28) has to be considered for cells $i$ only, for which $\mu_i$ is non-zero.

4. For the case that $R_{ji}$ and $t_{ji}$ do not depend on $j$, such that one can define $Z_i = R_i \mathrm{e}^{\gamma t_i}$ instead of Eq. (22), a consequence of the set of nonlinear equations is, $\sum_i Z_i \mu_i = 1$. This describes how the overall decay of the measure by the reflectivity $R_i$ is compensated by $\mathrm{e}^{\gamma t_i}$. It follows from summing Eq. (33) over $j$ together with Eqs. (32) and (34).

5. Note that Eq. (28) need not be included in the set of nonlinear equations, as it is equivalent to Eq. (32). This can be seen by multiplying Eq. (31) with the denominator of the r.h.s. and summing over $j$, leading to

$$\sum_j P_{ji} = \frac{1 - \left(\sum_j y_j \ P_{ji} Z_{ji}\right) \mu_i}{1 - \qquad y_i \qquad \mu_i} \quad \forall i \ . \tag{35}$$

# IV. NUMERICAL APPROACH FOR DETERMINING MEASURES

Depending on the decay rate $\gamma$ one has to use different methods for determining the corresponding conditionally invariant measure $\mu$. In case of the natural decay, one has first to determine the natural decay rate. For systems with partial escape this holds also for the inverse decay. In all cases, the result depends on the number $n$ of cells of the partition and should converge in the limit $n \to \infty$.

We provide Python code (as separate files) to compute $P^{\mathcal{L}}$, $P$, and $\mu$ with the presented methods for all four example systems of the main text.

## A. Natural decay rate

The approach to determine the natural decay rate $\gamma_{\text{nat}}$ and the natural measure $\mu_{\text{nat}}$ depends on the properties of the transition time $t_{ji}$.

### 1. *Transition time constant*

For systems where the transition time $t_{ji} = \text{const}$, like maps, one can directly diagonalize the eigenproblem given in the main text,

$$\sum_i P^{\mathcal{L}}_{ji} R_{ji}\, \mu_i = \mathrm{e}^{-\gamma}\, \mu_j \quad ; \quad j = 1, \dots, n \,, \tag{36}$$

with the Lebesgue transition matrix $P^{\mathcal{L}}_{ji}$. The leading eigenvalue $\mathrm{e}^{-\gamma}$ gives the natural decay rate $\gamma = \gamma_{\text{nat}}$ and the corresponding right eigenvector the natural measure $\mu = \mu_{\text{nat}}$. For solving the eigensystem one can use sparse matrix methods, as $P^{\mathcal{L}}_{ji}$ is sparse with the number of non-zero entries scaling just with $n$.

### 2. *Transition time not constant*

For systems where the transition time $t_{ji} \neq \text{const}$, like billiards, one has to find the natural decay rate $\gamma_{\text{nat}}$ and the coarse-grained measure $\mu_{\text{nat}}$ iteratively. We start from the eigenvalue problem given in the main text,

$$\sum_i P^{\mathcal{L}}_{ji} R_{ji} \mathrm{e}^{\gamma t_{ji}}\, \mu_i(\gamma) = \lambda(\gamma)\, \mu_j(\gamma) \quad ; \quad j = 1, \dots, n \,, \tag{37}$$

where we have added the leading eigenvalue $\lambda$ explicitly and use the Lebesgue transition matrix $P^{\mathcal{L}}_{ji}$. Here $\gamma$ has to be adjusted, such that $\lambda(\gamma) = 1$.

We use a Newton–Raphson method with initial guess $\gamma = 0$, which needs the derivative $\frac{\mathrm{d}\lambda}{\mathrm{d}\gamma}$. To this end we take the derivative of Eq. (37) with respect to $\gamma$, observing that both $\lambda$ and the measure $\mu$ depend on $\gamma$,

$$\sum_i P^{\mathcal{L}}_{ji} R_{ji} \mathrm{e}^{\gamma t_{ji}} \left( t_{ji}\, \mu_i(\gamma) + \frac{\mathrm{d}\mu_i(\gamma)}{\mathrm{d}\gamma} \right) = \frac{\mathrm{d}\lambda}{\mathrm{d}\gamma}\, \mu_j(\gamma) + \lambda\, \frac{\mathrm{d}\mu_j(\gamma)}{\mathrm{d}\gamma} \,. \tag{38}$$

Furthermore, we need the left leading eigenvector $\mu^{\mathrm{L}}_j$ of Eq. (37), given by,

$$\sum_j \mu^{\mathrm{L}}_j(\gamma)\, P^{\mathcal{L}}_{ji} R_{ji} \mathrm{e}^{\gamma t_{ji}} = \lambda(\gamma)\, \mu^{\mathrm{L}}_i(\gamma) \qquad i = 1, \dots, n \,. \tag{39}$$

Now we multiply Eq. (38) with $\mu^{\mathrm{L}}_j$ and sum over $j$, such that two terms cancel, giving

$$\sum_{i,j} \mu^{\mathrm{L}}_j(\gamma)\, P^{\mathcal{L}}_{ji} R_{ji} t_{ji} \mathrm{e}^{\gamma t_{ji}}\, \mu_i(\gamma) = \frac{\mathrm{d}\lambda}{\mathrm{d}\gamma} \sum_j \mu^{\mathrm{L}}_j(\gamma)\, \mu_j(\gamma) \,. \tag{40}$$

Finally, this gives the derivative of the leading eigenvalue $\lambda$ with respect to $\gamma$,

$$\frac{\mathrm{d}\lambda}{\mathrm{d}\gamma} = \frac{\sum_{i,j} \mu^{\mathrm{L}}_j(\gamma)\, P^{\mathcal{L}}_{ji} R_{ji} t_{ji} \mathrm{e}^{\gamma t_{ji}}\, \mu_i(\gamma)}{\sum_j \mu^{\mathrm{L}}_j(\gamma)\, \mu_j(\gamma)} \,. \tag{41}$$

### B. Inverse natural decay rate

For systems with partial escape the determination of the inverse natural decay rate $\gamma_{\text{inv}}$ and the inverse natural measure $\mu_{\text{inv}}$ occur in analogy to the natural decay.

One has to determine the Lebesgue transition matrix from the inverse dynamics, i.e. from dynamics backward in time and using the inverse of the reflectivities and combine them in backward order. Using this Lebesgue transition matrix one can follow the approach for the natural decay depending on the properties of the transition time $t_{ji}$.

The step of determining the Lebesgue transition matrix of the inverse dynamics can be replaced by using the original transition matrix $P^{\mathcal{L}}_{ji}$ and doing one of the following:

1. Transpose the Lebesgue transition matrix $\bar{P}^{\mathcal{L}}_{ij} = P^{\mathcal{L}}_{ji}$. The problem is, that if the original Lebesgue transition matrix $P^{\mathcal{L}}_{ji}$ is approximated numerically by a finite number of trajectories, typically the sum $\sum_i P^{\mathcal{L}}_{ji} \neq 1$ and thus $\sum_j \bar{P}^{\mathcal{L}}_{ji} \neq 1$. However, this is required by the algorithm for arbitrary decay rates. This can be solved by normalizing $\bar{P}^{\mathcal{L}}_{ji}$ correspondingly. This will introduce an error that is of the same order as the already existing error due to the numerical approximation of the Lebesgue transition matrix.

2. If the closed system is time-reversal symmetric and the reflectivities are independent on the sign of the momentum $p$, one can use the original Lebesgue transition matrix $P^{\mathcal{L}}_{ji}$. The forward dynamics at momentum $-p$ corresponds to the backward dynamics at momentum $p$. One just has to mirror the final measure with respect to the sign of $p$.

### C. Arbitrary decay rate

One has to numerically find a solution to the set of nonlinear Eqs. (31) to (34) for a desired value of $\gamma$. As the number of unknown variables is quite large, standard algorithms for nonlinear sets of equations do not work. Instead, we present two iterative algorithms described below.

#### 1. *Iterative algorithm for* $\gamma \in (\gamma_{nat}, \gamma_{inv})$

This iterative algorithm works for $\gamma \in (\gamma_{\text{nat}}, \gamma_{\text{inv}})$ (partial escape) and $\gamma > \gamma_{\text{nat}}$(full escape). The algorithm is slow near the boundary.

0. Initialize: $\mu_i = \mu_i^{\text{nat}}$ , $y_i = n \cdot 10^{-6}$.

1. Determine $P_{ji}$ from Eq. (31).

2. Determine $\mu'_i$ by evaluating the l.h.s. of Eq. (33).

3. Determine $P_{ji}$ from Eq. (31) now using $\mu'_i$.

4. Multiply $\mu'_i$ with l.h.s. of Eq. (32), $\mu''_i = \mu'_i \ \sum_j P_{ji}$.

5. Update $y'_i = y_i + \frac{1}{\mu''_i} - \frac{1}{\mu'_i} = y_i + \frac{1-\sum_j P_{ji}}{\mu''_i}$
(Motivation: In Eq. (31) just the term with $y_j$ should be affected and not the other terms when $P_{ji}\mu_i$ is evaluated the next time. Thus the other terms $\frac{1}{\mu'_i} - y_i$ should be unchanged when the new variables $\mu''_i$ and $y'_i$ are used, i.e. $\frac{1}{\mu'_i} - y_i = \frac{1}{\mu''_i} - y'_i$. This reasoning becomes more transparent when working with $\mu_{ji} = P_{ji}\mu_i$ rather than with $P_{ji}$.)

6. Rename $\mu''_i$ and $y'_i$ to $\mu_i$ and $y_i$, respectively.

7. Determine norm $\mathcal{N} = \sum_i \mu_i$, divide $\mu_i$ by $\mathcal{N}$ to fulfill Eq. (34), and multiply $y_i$ by $\mathcal{N}$ such that Eq. (31) remains fulfilled.

8. Return to step 1, unless the change in $\mu_i$ compared to the last iteration is sufficiently small.

### 2. Iterative algorithm for $\gamma < \gamma_{nat}$

This iterative algorithm works for $\gamma \approx \gamma_{\rm nat}$, in particular it works for $\gamma < \gamma_{\rm nat}$. For increasing number $n$ of Ulam cells the range of convergence around $\gamma_{\rm nat}$ becomes smaller. Factorize $y_i = \mathcal{N}\,\tilde{y}_i$ with $\mathcal{N}$ the norm and $\sum_i \tilde{y}_i = 1$.

0. Initialize: $\mu_i = 1/n$ and $\mathcal{N} \equiv 0$ (corresponds to $\gamma_{\rm nat}$).

1. Determine $P_{ji}$ from Eq. (31).

2. Solve eigenvalue problem of $\mu_i$ with Eqs. (33) and (34). Note that it is faster to apply the matrix about 20 times to the previous approximation of the measure. This uses the fact that we are searching for the leading eigenvector.

3. Solve eigenvalue problem of $\tilde{y}_i$ with Eq. (28) instead of the equivalent Eq. (32). Normalize such that $\sum_i \tilde{y}_i = 1$. See comment on matrix application as in previous step.

4. If the eigenvalue of Eqs. (33) and (28), here called $\lambda$, is not 1, we adapt $\mathcal{N}$ iteratively:

$$\mathcal{N}' = \mathcal{N} + \frac{1-\lambda}{\frac{\mathrm{d}\lambda}{\mathrm{d}\mathcal{N}}} \tag{42}$$

$$\frac{\mathrm{d}\lambda}{\mathrm{d}\mathcal{N}} = \frac{\sum_{i,j} \tilde{y}_j \frac{\mathrm{d}P_{ji}}{\mathrm{d}\mathcal{N}} Z_{ji}\mu_i}{\sum_j \tilde{y}_j \mu_j} \tag{43}$$

$$\frac{\mathrm{d}P_{ji}}{\mathrm{d}\mathcal{N}} = -\frac{P_{ji}^{\mathcal{L}}\,(\tilde{y}_j Z_{ji} - \tilde{y}_i)\,\mu_i}{(1+\mathcal{N}\,(\tilde{y}_j Z_{ji} - \tilde{y}_i)\,\mu_i)^2} \tag{44}$$

This follows from taking the derivative of Eq. (33) (with $\lambda(\mathcal{N})$ added on the r.h.s) with respect to $\mathcal{N}$ and applying $\sum_j \tilde{y}_j$ on both sides. Using Eq. (28) and $\lambda = 1$ the terms with $\frac{\mathrm{d}\mu_i}{\mathrm{d}\mathcal{N}}$ cancel.

## D. Measure in position space

In the previous sections we describe how to determine the measure in the boundary phase space. However, for time-continuous systems a comparison in position space is desirable too, see Fig. 1 (main text) and Figs. S2(b), S4(b), S10(b), and S11(b). To this end, we extrapolate the measure from the boundary to position space using rays.

For the three-disk scattering system a random initial condition $(s,p)$ in the boundary phase space is chosen and evolved along a ray in position space until the next collision with the boundary. Rays leaving the system, i.e. with no further collision with a boundary, are taken until some cutoff in position space. On each ray several points $(x_i, y_i)$ are randomly chosen with a fixed line density, i.e. the number of points is proportional to the length of the ray. Let $t(x_i, y_i)$ be the time from the boundary point $(s,p)$ to $(x_i, y_i)$ and $\mu(s,p)$ the measure of the corresponding partition cell on the boundary phase space. Then to each point $(x_i, y_i)$ we assign a weight $w(x_i, y_i) = \mathrm{e}^{\gamma t(x_i,y_i)}\mu(s,p)$. The exponential increase with $t$ preserves conditional invariance in position space. This is repeated for many random initial conditions chosen uniformly in the boundary phase space. In summary, to many points in position space we assign a weight, that is obtained by selecting many initial conditions and several points on each ray. The measure in position space is then given by a position-space histogram of all these weights, which is suitably normalized.

For dielectric cavities with refractive index $n_{\rm r}$ inside of the cavity the procedure is similar. However, additionally to the reflected ray of each selected initial point on the boundary phase space $(s,p)$, the incoming and the transmitted rays are also considered:

- Reflected ray: The weight of a point $(x_i, y_i)$ is given by $w(x_i, y_i) = R^{\rm TM/TE}(p)\,\mathrm{e}^{\gamma n_{\rm r} t(x_i,y_i)}\mu(s,p)$. Here, $R^{\rm TM/TE}(p)$ is the Fresnel reflection coefficient [1], which depends on the chosen polarization, see Sec. I A. The refractive index $n_{\rm r}$ is used to account for the slower in-medium speed of light inside the cavity.

- Incoming ray: The weight is given by $w(x_i, y_i) = \mathrm{e}^{\gamma n_{\rm r} t(x_i,y_i)}\mu(s,p)$, but here the time $t$ is negative.

- Transmitted ray: It is only considered if there is no total internal reflection at $(s,p)$. The weight is given by $w(x_i, y_i) = \sqrt{\frac{1-n_{\rm r}^2p^2}{1-p^2}}\,T^{\rm TM/TE}(p)\,\mathrm{e}^{\gamma t(x_i,y_i)}\mu(s,p)$. Here, $T^{\rm TM/TE}(p)$ is the Fresnel transmission coefficient. The square root factor compensates the increased ray density after transmission by decreasing the weight. Reentrance of some transmitted rays back into the cavity, which occurs in non-convex cavities, is not considered for simplicity.

Finally, the measure in position space is again given by a position-space histogram of all these weights. Note, however, that the contribution from rays inside the cavity has been counted twice as we consider incoming and reflected rays. One therefore has to divide the weight of each bin inside the cavity in the position-space histogram by a factor of two, before suitable normalization.

We provide Python code (as separate files) to compute the measure in position space with the presented method for the three-disk scattering system and dielectric cavities.

## V. REFERENCES


[1] H. Cao and J. Wiersig, *Dielectric microcavities: Model systems for wave chaos and non-Hermitian physics*, Rev. Mod. Phys. **87**, 61 (2015).

[2] R. Ketzmerick, K. Clauß, F. Fritzsch, and A. Bäcker, *Chaotic resonance modes in dielectric cavities: Product of conditionally invariant measure and universal fluctuations*, Phys. Rev. Lett. **129**, 193901 (2022).

[3] J. R. Schmidt and R. Ketzmerick, *Resonance states of the three-disk scattering system*, New J. Phys. **25**, 123034 (2023).

[4] B. V. Chirikov, *A universal instability of many-dimensional oscillator systems*, Phys. Rep. **52**, 263 (1979).

[5] M. V. Berry, N. L. Balazs, M. Tabor, and A. Voros, *Quantum maps*, Ann. Phys. (N.Y.) **122**, 26 (1979).

[6] S.-J. Chang and K.-J. Shi, *Evolution and exact eigenstates of a resonant quantum system*, Phys. Rev. A **34**, 7 (1986).

[7] K. Clauß and R. Ketzmerick, *Local random vector model for semiclassical fractal structure of chaotic resonance states*, J. Phys. A **55**, 204006 (2022).

[8] T. A. Brody, J. Flores, J. B. French, P. A. Mello, A. Pandey, and S. S. M. Wong, *Random-matrix physics: spectrum and strength fluctuations*, Rev. Mod. Phys. **53**, 385 (1981).

[9] S. Nonnenmacher and A. Voros, *Chaotic eigenfunctions in phase space*, J. Stat. Phys. **92**, 431 (1998).

[10] A. Bäcker, *Numerical aspects of eigenvalues and eigenfunctions of chaotic quantum systems*, in M. Degli Esposti and S. Graffi (editors) "The Mathematical Aspects of Quantum Maps", volume 618 of *Lect. Notes Phys.*, 91, Springer-Verlag, Berlin (2003).

[11] K. Clauß, E. G. Altmann, A. Bäcker, and R. Ketzmerick, *Structure of resonance eigenfunctions for chaotic systems with partial escape*, Phys. Rev. E **100**, 052205 (2019).
